# Supplementary material for: Self-consistent gyrokinetic modelling of turbulent and neoclassical tungsten transport in toroidally rotating plasmas
Source: arXiv:2304.12603 source file (2023-04-25)
Supplement: Supplementary file 1 [file 8_Appendix.tex]

\section{Impurity density distribution from the parallel dynamics}\label{Ch5:appendix}
In the case of the large aspect ratio $(\epsilon \ll 1)$ and for a circular cross section, the normalized magnetic field $b= 1/(1-\epsilon \cos\theta)$, the impurity density $N$ and the Mach number $M$ can be expanded in $\epsilon$ 
\begin{align}
    b^2 &= 1-2\epsilon \cos\theta + \mathcal{O}(\epsilon^2), \label{b} \\
    N &= 1+N_c \cos\theta + N_s\sin \theta + \mathcal{O}(\epsilon^2), \label{density2}\\
    M^2 &= M_0^2(1+2\epsilon \cos\theta)+\mathcal{O}(\epsilon^2). \label{Mach}
\end{align}

By using the quasi-neutrality constraint and the modified Mach number Eq. (\ref{Eq:modified_mach_number}), the initial parallel impurity transport Eq. (\ref{Ch5_parallel_2}) can be expressed as \cite{Fulop1999}
\begin{align}
    (1+\alpha N)\frac{\partial N}{\partial \vartheta} = \mathrm{g}(n-b^2+\gamma(N-\langle Nb^2\rangle)b^2) + N\frac{\partial M^2}{\partial \vartheta} - \Bigg\langle N\frac{\partial M^2}{\partial \vartheta}\Bigg\rangle b^2,
\label{density_eq3}
\end{align}
where we introduced $\alpha=\langle N_z \rangle Z^2 T_0(2 N_0 T_i)$ with $2N_0/T_0 = N_{e0}/T_e + N_{i0}/T_i$

In order to find the expression for \textit{'up-down'} and \textit{'in-out'} asymmetric parameters derived in Eqs. (\ref{Eq:Fulop_ud}, \ref{Eq:Fulop_io}), we insert Eqs. (\ref{b} -\ref{Mach}) into Eq. (\ref{density_eq3}), which writes
\begin{align}
    \cos\theta\bigg(gN_c(1+\gamma)-N_s(1+\alpha)+2\mathrm{g}\epsilon\bigg) + \sin\theta\bigg(gN_s(1+\gamma)+N_c(1+\alpha)-2\epsilon M_0^2 \bigg) = 0,
\end{align}
where we have neglected all the higher order terms $\epsilon^2, n_c\epsilon, N_s\epsilon \sim \mathcal{O}(\epsilon^2)$. 

This last equation should be satisfied with all the different angles $\theta$, therefore each coefficient of $\cos\theta$ and $\sin\theta$ should be equal to zero.
\begin{align}
    gN_c(1+\gamma)-N_s(1+\alpha)+2\mathrm{g}\epsilon &= 0 \label{density_eq4} \\
    gN_s(1+\gamma)+N_c(1+\alpha)-2\epsilon M_0^2 &=0 \label{density_eq5}
\end{align}
By arranging both Eq.(\ref{density_eq4}, \ref{density_eq5}), we can finally obtain the \textit{'up-down'} asymmetry term $N_s$ and \textit{'in-out'} asymmetry term $N_c$
\begin{align}
    N_c &= 2\epsilon \frac{(1+\alpha)M_0^2 -(1+\gamma)g^2}{(1+\alpha)^2+(1+\gamma)^2g^2} \qquad \text{('in-out')} \\
    N_s &= 2\epsilon \mathrm{g} \frac{(1+\alpha)+(1+\gamma)M_0^2}{(1+\alpha)^2+(1+\gamma)^2g^2} \qquad \text{('up-down')}
\end{align}
In the trace limit of impurities ($N_z Z^2 \ll 1$), these equations can be further simplified since $\alpha \ll 1$ : 
\begin{align}
    N_c &= 2\epsilon \frac{M_0^2 -(1+\gamma)g^2}{1+(1+\gamma)^2g^2} \qquad \text{('in-out')} \\
    N_s &= 2\epsilon \mathrm{g} \frac{1+(1+\gamma)M_0^2}{1+(1+\gamma)^2g^2} \qquad \text{('up-down')}
\end{align}
Note that the toroidal rotation causes the impurities to accumulate on the outside of the flux surface, which will enhances the neoclassical impurity transport.
